# Supplementary material for: What you lose when you snooze: how duty cycling impacts on the contact process in opportunistic networks
Source: arXiv:1709.09551 ancillary file (2017-09-28)
Supplement: Supplementary file 1 [file supplemental_material.pdf]

# What you lose when you snooze: how duty cycling impacts on the contact process in opportunistic networks

Elisabetta Biondi, Chiara Boldrini,  
Andrea Passarella, Marco Conti\*

## A Proofs and further results for the negligible contact duration case

### A.1 Why the measured contact process is not renewal

In general, the distribution of  $N_j$  is a function of everything that has happened before the last detected contact at  $\tilde{X}_{j-1}$ . In fact,  $N_j$  counts the missed contacts starting from the time of the last detected contact, which in turn depends on the time of the contact before that one, and so on and so forth. Hence, for  $\tilde{S}_j$  the following proposition holds.

**Proposition 1.** *Since  $N_j$  are not i.i.d. for all  $j$ , the measured intercontact times  $\tilde{S}_j$  are not i.i.d. in general and the measured contact process is not a renewal process.*

*Proof.* Recalling that  $S_i$  are i.i.d. by definition, if  $N_j$  were i.i.d. for all  $j$  and independent of the inter-contact times  $S_i$  occurred before the  $(j-1)$ -th detected contact, then also  $\tilde{S}_j$  would be i.i.d. and the detected contact process could be treated as a renewal process. Unfortunately, this is not the case. In fact, after noticing that  $N_j$  is equal to  $k$  only if the first  $k-1$  contacts are missed and the  $k$ -th is detected, the PDF of  $N_j$  can be written as follows:

$$\mathbb{P}(N_j = k) = \prod_{z=1}^{k-1} \mathbb{P} \left( \tilde{X}_{j-1} + \sum_{v=1}^z S_v \notin \bigcup_{v=\tilde{n}_{j-1}}^{\infty} \mathcal{I}_v^{ON} \right) \mathbb{P} \left( \tilde{X}_{j-1} + \sum_{v=1}^k S_v \in \bigcup_{v=\tilde{n}_{j-1}}^{\infty} \mathcal{I}_v^{ON} \right), \quad (\text{A.1})$$

where the first  $k-1$  factors denote the joint probability that none of the first  $k-1$  contacts fall into any ON interval (recall that  $\bigcup_{v=\tilde{n}_{j-1}}^{\infty} \mathcal{I}_v^{ON}$  is the set of all ON intervals after the  $\tilde{n}_{j-1}$ -th) and the  $k$ -th term gives instead the probability that the  $k$ -th contact is detected. Equation A.1 shows that the distribution of  $N_j$  is a function of everything that has happened before the  $\tilde{n}_{j-1}$ -th contact. In fact,  $\tilde{X}_{j-1}$  can be rewritten as  $\tilde{X}_{j-2} + \tilde{S}_{j-1}$ , where  $\tilde{X}_{j-2}$  is the time at which the previous detected contact took place and is given by the sum of  $N_{j-1}$  intercontact times. Hence  $N_j$  and  $N_{j-1}$  are not independent and, in turn,  $\tilde{S}_j$  are not i.i.d.  $\square$

### A.2 Proof of Lemma 1

*Proof.* Since  $\tilde{n}_{j-1}$  denotes the ON interval in which the  $(j-1)$ -th detected contact takes places, we can rewrite  $\tilde{X}_{j-1}$  as  $\tilde{n}_{j-1}T + Z_{j-1}^{ON}$ , where we have denoted with  $Z_{j-1}^{ON}$  the displacement of the detected contact within the ON interval. If we substitute this expression of  $\tilde{X}_{j-1}$  in Equation A.1,

---

\*All authors are with IIT-CNR, Via G. Moruzzi 1, Pisa, Italy

we obtain the following:

$$\begin{aligned} \prod_{z=1}^{k-1} \mathbb{P} \left( \tilde{n}_{j-1}T + Z_{j-1}^{ON} + \sum_{v=1}^z S_v \notin \bigcup_{v=\tilde{n}_{j-1}}^{\infty} \mathcal{I}_v^{ON} \right) \mathbb{P} \left( \tilde{n}_{j-1}T + Z_{j-1}^{ON} + \sum_{v=1}^k S_v \in \bigcup_{v=\tilde{n}_{j-1}}^{\infty} \mathcal{I}_v^{ON} \right) = \\ = \prod_{z=1}^{k-1} \mathbb{P} \left( Z_{j-1}^{ON} + \sum_{v=1}^z S_v \notin \bigcup_{v=0}^{\infty} \mathcal{I}_v^{ON} \right) \mathbb{P} \left( Z_{j-1}^{ON} + \sum_{v=1}^k S_v \in \bigcup_{v=0}^{\infty} \mathcal{I}_v^{ON} \right), \quad (\text{A.2}) \end{aligned}$$

where the last equality is obtained operating a shift of the index  $\tilde{n}_{j-1}$  of ON intervals (in other words, we start counting from the  $\tilde{n}_{j-1}$ -th interval, which becomes  $[0, \tau)$  in our shifted reference system). We now want to find under which conditions  $Z_{j-1}^{ON}$  is independent of the history of the contact process. Let us assume, without loss of generality, that the previous contact (whether detected or not) took place at  $t^*$  (which, after the shift, is negative). Then,  $Z_{j-1}^{ON}$  is equivalent to  $t^* + S$  under the constraint that  $t^* + S$  falls into an ON interval (i.e. the contact is detected). This can be cast, applying the formulas for conditional probabilities, into the following expression:

$$\mathbb{P}(Z_{j-1}^{ON} > z) = \mathbb{P}(\tau > t^* + S > z | \tau > t^* + S > 0) = \frac{P(\tau - t^* > S > z - t^*)}{P(\tau - t^* > S > -t^*)}. \quad (\text{A.3})$$

It is easy to see that, when the PDF of  $S$  (which we denote as  $f_S$ ) is slowly varying (i.e. approximately flat) in intervals of length  $\tau$ , the ratio in the previous equation corresponds to the ratio of the areas below the PDF. Thus, we obtain the following:

$$\mathbb{P}(Z_{j-1}^{ON} > z) \sim \frac{(\tau - z) \cdot f_S(\tau - t^*)}{\tau \cdot f_S(\tau - t^*)} = \frac{(\tau - z)}{\tau} \quad (\text{A.4})$$

The above proves that whatever the time  $t^*$  of the previous contact, if the PDF of  $S$  is slowly varying in intervals of length  $\tau$ , then  $Z_{j-1}^{ON}$  would be uniformly distributed and independent of the previous evolution of the contact process. This concludes the proof.  $\square$

### A.3 Applicability of Lemma 1 and Lemma 2 under specific distributions

Before concluding this section, we analyse in which cases the assumption in Lemma 1 and Lemma 2 about the slowly varying nature of  $f_S$  is reasonable. Since in the rest of the paper we will use Lemma 1 and Lemma 2 simultaneously, we require  $f_S$  to be slowly varying in intervals of size  $\max\{\tau, T - \tau\}$ , which can be translated into the sufficient condition of  $f_S$  being slowly varying in intervals of size  $T$ .

We consider two popular assumptions for the distribution of the intercontact times, namely the exponential and Pareto<sup>1</sup> distributions [2, 6, 9]. Let us start with exponentially distributed intercontact times, whose rate we denote with  $\lambda = \frac{1}{\mathbb{E}[S]}$ . The PDF  $f_S(x) = \lambda e^{-\lambda x}$  of the intercontact time  $S$  is thus a positive, strictly decreasing convex function for  $x > 0$ . Hence, if we prove that  $f_S(x)$  is slowly varying in the first interval of length  $T$ , i.e. in  $[0, T]$ , we are sure that the same holds true also for the next intervals. For  $f_S(x)$  to be slowly varying in  $[0, T]$ , we need  $\frac{f_S(0)}{f_S(T)} \sim 1$ , which is equivalent to  $\frac{f_S(0)}{f_S(T)} = \frac{\lambda e^{-\lambda 0}}{\lambda e^{-\lambda T}} = \frac{1}{e^{-\lambda T}}$ . Thus, when sufficient condition  $\lambda T \ll 1$  holds, Lemma 1 also holds.

When intercontact times are Pareto, we have  $f_S(x) = \frac{\alpha b^\alpha}{(b+x)^{\alpha+1}}$ . The PDF is strictly decreasing and convex also in this case, so we can again focus on  $[0, T]$ . Following the same line of reasoning as above, we obtain condition  $T \ll b$  (which is equivalent to  $\frac{T}{\mathbb{E}[S](\alpha-1)} \ll 1$  when  $\alpha > 1$ ).

### A.4 Proof of Theorem 1

*Proof.* Let us start from case  $N = 1$ . As illustrated in Figure A1, the following equalities hold:

$$\mathbb{P}\{N = 1\} = \mathbb{P}\{E_1 = 1\} = \sum_{n_1=0}^{\infty} \mathbb{P}(X_1 \in \mathcal{I}_{n_1}^{ON}) = \sum_{n_1=0}^{\infty} \mathbb{P}(\tilde{X}_0 + S_1 \in \mathcal{I}_{n_1}^{ON}), \quad (\text{A.5})$$

<sup>1</sup>For convenience of manipulation, we use the American version of the Pareto distribution, as in [1, 7]

where  $\tilde{X}_0$  as usual denotes the time at which the last contact has been detected. Exploiting Lemma 1 (hence assuming that  $f_S$  is slowly varying in any interval of length  $\tau$ ), we can rewrite  $\tilde{X}_0$  as  $Z^{ON} \sim \text{Unif}(0, \tau)$ . Then, the sum  $Z^{ON} + S_1$  is well defined, and its probability density can be derived as the convolution of the densities of  $Z^{ON}$  and  $S$ . For the sake of convenience, in the following we use  $g$  to indicate the probability  $\mathbb{P}\{N = 1\} = \sum_{n_1=0}^{\infty} \mathbb{P}(Z^{ON} + S \in \mathcal{I}_{n_1}^{ON})$ .

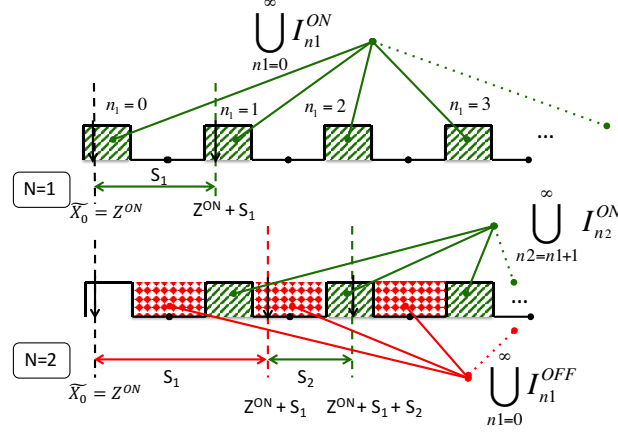

Figure A1: Examples for case  $N = 1$  and  $N = 2$ .

Let us now consider case  $N = 2$ , which means that the first contact is missed and the second one is detected, i.e.  $P\{N = 2\} = \mathbb{P}\{E_1 = 0, E_2 = 1\}$ . In this case, we have the following:

$$P\{N = 2\} = \sum_{n_1=0}^{\infty} \mathbb{P}(X_1 \in \mathcal{I}_{n_1}^{OFF}) \left( \sum_{n_2=n_1+1}^{\infty} \mathbb{P}(X_2 \in \mathcal{I}_{n_2}^{ON}) \right) \quad (\text{A.6})$$

Exploiting the property of conditional probabilities, the second term at the right-hand side of the above equation can be rewritten as follows:

$$\sum_{n_2=n_1+1}^{\infty} \mathbb{P}(X_2 \in \mathcal{I}_{n_2}^{ON}) = \sum_{n_2=n_1+1}^{\infty} \mathbb{P}(X_1 + S_2 \in \mathcal{I}_{n_2}^{ON} | X_1 \in \mathcal{I}_{n_1}^{OFF}) \quad (\text{A.7})$$

$$= \sum_{n_2=n_1+1}^{\infty} \mathbb{P}(Z^{OFF(n_1)} + S_2 \in \mathcal{I}_{n_2}^{ON}) \quad (\text{A.8})$$

$$= \sum_{n_2=1}^{\infty} \mathbb{P}(Z^{OFF} + S_2 \in \mathcal{I}_{n_2}^{ON}). \quad (\text{A.9})$$

In Equation A.7 we have conditioned on the first contact falling into an OFF interval, which follows from the first term at the right-hand side of Equation A.6. Then, we go from Equation A.7 to Equation A.8 applying Lemma 2 (hence assuming that  $f_S$  is slowly varying in any interval of length  $T - \tau$ ) and denoting with  $Z^{OFF(n_1)}$  a random variable uniformly distributed in  $\mathcal{I}_{n_1}^{OFF}$ . Finally, Equation A.8 is then shifted by  $n_1$ . Now, the summation in  $n_2$  does not depend on what happens to the previous contacts and it is only a function of  $S_2$  and the duty cycling parameters  $\tau$  and  $T$ . For the convenience of notation, in the following we use  $p$  to synthetically denote probability  $\sum_{n_2=1}^{\infty} \mathbb{P}(Z^{OFF} + S_2 \in \mathcal{I}_{n_2}^{ON})$ .

In order to conclude the proof for case  $N = 2$ , let us go back to the right-hand side of Equation A.6. We have just derived the second term, now we have to study the first term  $\sum_{n_1=0}^{\infty} \mathbb{P}(X_1 \in \mathcal{I}_{n_1}^{OFF})$ . Quantity  $\sum_{n_1=0}^{\infty} \mathbb{P}(X_1 \in \mathcal{I}_{n_1}^{OFF})$  corresponds to the probability that the first contact does not fall into an ON interval, hence corresponds to  $1 - \mathbb{P}\{N = 1\}$ , which is given by  $1 - g$ . Putting everything together, we have that  $\mathbb{P}\{N = 2\} = (1 - g)p$ .

For  $N = 3$  the line of reasoning is similar. The only difference is that the sequence of events is now missed-missed-detected, i.e.  $P\{N = 3\} = \mathbb{P}\{E_1 = 0, E_2 = 0, E_3 = 1\}$ . For the sake of tractability, we neglect the probability that two missed contacts happen in the same OFF

interval (under the conditions in Lemma 1 and Lemma 2, this probability would be very low anyway<sup>2</sup>). Then, we obtain the following:

$$P\{N = 3\} = \sum_{n_1=0}^{\infty} \mathbb{P}(X_1 \in \mathcal{I}_{n_1}^{OFF}) \left[ \sum_{n_2=n_1+1}^{\infty} \mathbb{P}(X_2 \in \mathcal{I}_{n_2}^{OFF}) \left( \sum_{n_3=n_2+1}^{\infty} \mathbb{P}(X_3 \in \mathcal{I}_{n_3}^{ON}) \right) \right] \quad (\text{A.10})$$

Again, we want to make the three summations independent. It is easy to see that  $\sum_{n_3=n_2+1}^{\infty} \mathbb{P}(X_3 \in \mathcal{I}_{n_3}^{ON})$  can be manipulated exactly as  $\sum_{n_2=n_1+1}^{\infty} \mathbb{P}(X_2 \in \mathcal{I}_{n_2}^{ON})$  in the case  $\mathbb{P}\{N = 2\}$  (see Equation A.7 and following), obtaining again  $p$ . As for the second summation, equality  $\sum_{n_2=n_1+1}^{\infty} \mathbb{P}(X_2 \in \mathcal{I}_{n_2}^{OFF}) = \sum_{n_2=n_1+1}^{\infty} 1 - \mathbb{P}(X_2 \in \mathcal{I}_{n_2}^{ON})$  holds, which can be rewritten as  $1 - p$ . The first summation, which is now independent of the other two, is again equal to  $1 - \mathbb{P}\{N = 1\} = 1 - g$ , from which  $\mathbb{P}\{N = 3\} = (1 - g)(1 - p)p$ . Generalising this result to the case  $N = k$ , we obtain Equation 2.

Before concluding the proof, several remarks need to be made. First, note that we have to separate the first contact from the others that follow because the first contact happens, by definition, after a detected contact (which takes place in  $\mathcal{I}_n^{ON}$ ), while all others follow a missed contact (which happens in  $\mathcal{I}_n^{OFF}$ ). Also note that since we are applying both Lemma 1 and Lemma 2 we need  $f_S$  to be slowly varying in any of the largest ON/OFF intervals, so we take  $\max\{\tau, T - \tau\}$ . However,  $g$  depends on Lemma 1 only, while  $p$  depends on Lemma 2 only. This implies that when  $\tau < T/2$  the value of  $g$  tends to be more accurate than that of  $p$ , while the opposite holds true when  $\tau > T/2$ .  $\square$

## A.5 Proof of Corollary 2

Let us consider  $g$  and  $p$  as defined in Theorem 1. Probability  $g$  depends on  $Z^{ON}$ , while probability  $p$  depends on  $Z^{OFF}$ . We first focus on  $p$ , recalling that it can be obtained as follows:

$$p = \sum_{n_2=1}^{\infty} \frac{1}{T - \tau} \int_0^{T-\tau} \mathbb{P}(\tau + z + S_2 \in \mathcal{I}_{n_2}^{ON}) dz.$$

The integral in this expression corresponds to the shaded orange area in Figure A2. In fact, intervals of type  $\mathcal{I}_i^{ON} - \tau - z$  can be written as  $[iT - \tau - z, iT - z)$ . Similarly, recalling the expression  $g = \sum_{n_1=1}^{\infty} \frac{1}{\tau} \int_0^{\tau} \mathbb{P}(z + S_1 \in \mathcal{I}_{n_1}^{ON}) dz$ , we obtain that the integral in this expression corresponds to the blue area in Figure A2.

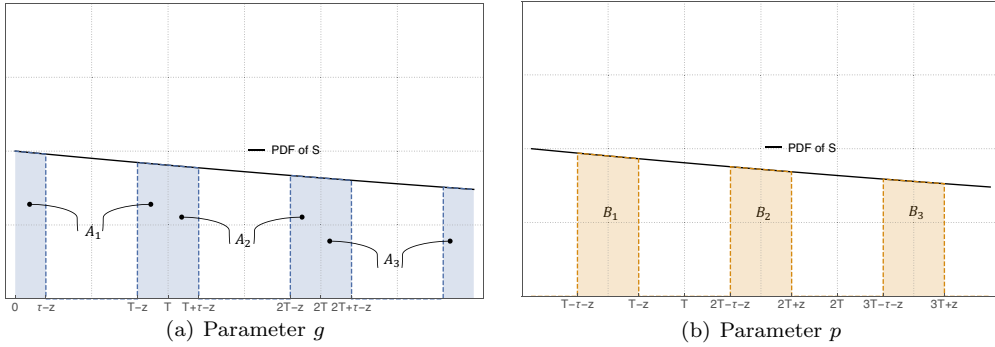

Figure A2: How to derive  $g$  and  $p$ .

Let us denote with  $A_n$  and  $B_n$  the areas within the  $n$ -th duty cycling interval for  $g$  and  $p$ , respectively. When  $f_S$  is slowly varying in intervals of length  $T$ , they can be rewritten as  $A_n = f_S(nT)(\tau - z) + f_S(nT)z = \tau f_S(nT)$  and  $B_n = \tau f_S(nT)$ , from which it follows that  $A_n = B_n$ , and neither of them depends on  $z_1$  and  $z_2$ . Thus, we can write  $g = p = \sum_{n=0}^{\infty} \tau f_S(nT)$ . Now let

<sup>2</sup>This can be easily seen, e.g., when real intercontact times are exponential with rate  $\lambda$ . In this case, the expected number of events in intervals of length  $T - \tau$  would be  $\lambda(T - \tau)$ , which is much smaller than 1 under our assumption.

us define  $C_n$  as the whole area under  $f_S(x)$  in the  $n$ -th duty cycling interval. It is straightforward to derive that  $C_n = T f_S(nT)$ . Using the expressions so far derived, the ratio  $\frac{\sum_n \tau f_S(nT)}{\sum_n T f_S(nT)}$  becomes equal to  $\frac{\tau}{T}$ . By definition of PDF,  $\sum_n C_n \sim 1$ , which implies that  $\sum_n \tau f_S(nT) \sim \frac{\tau}{T}$ , from which  $g \sim \frac{\tau}{T}$  follows.

## A.6 PMF of $N$ when intercontact times are exponential

**Theorem 1** (PMF of  $N$  when  $S \sim \text{Exp}(\lambda)$ ). *When intercontact times  $S_i$  are exponential with rate  $\lambda$ , the probability mass function of  $N$  can be obtained as follows:*

$$\begin{aligned} \mathbb{P}\{N = 1\} &= \frac{\lambda\tau - (1 - e^{-\lambda\tau})}{\lambda\tau} + \frac{1 - e^{-\lambda\tau}}{\lambda\tau} * \mathbb{P}(N^* = 1) \\ \mathbb{P}\{N = k\} &= \frac{1 - e^{-\lambda\tau}}{\lambda\tau} * \mathbb{P}(N^* = k), \quad k \geq 2 \end{aligned} \quad (\text{A.11})$$

where

$$\begin{aligned} \mathbb{P}\{N^* = 1\} &= \frac{1 - e^{-\lambda\tau}}{1 - e^{-\lambda T}} \\ \mathbb{P}\{N^* = k\} &= Li_{1-k}(e^{-\lambda T}) \frac{[\lambda(T - \tau)]^{k-1} (e^{\lambda\tau} - 1)}{(k-1)!}, \quad k \geq 2 \end{aligned} \quad (\text{A.12})$$

and  $Li_s(z)$  denotes the polylogarithm function ( $Li_s(z) = \sum_{k=1}^{\infty} \frac{z^k}{k^s}$ ).

*Proof.* When intercontact times  $S_i$  are exponential with rate  $\lambda$  the contact process becomes a Poisson Point Process. A useful property of Poisson Point Processes with rate  $\lambda$  is that the number of events occurring in an interval  $(a, b]$  is Poisson distributed with parameter  $\lambda(b - a)$ . When  $\lambda$  is large with respect to  $\tau$  we typically observe a burst of contacts in an ON interval. We define  $N^*$  as the number of contacts, *after the last one in the burst*, needed in order to detect the next one. Then, probability  $\mathbb{P}(N^* = 1)$  can be obtained, considering all intervals  $i$  in which the contact can be detected, as the probability that no contact occurred in the OFF and ON intervals before the  $i$ -th times the probability that a contact occurred in the  $i$ -th. Exploiting the property of Poisson Point Processes discussed above, we obtain  $\mathbb{P}(N^* = 1) = \sum_{i=1}^{\infty} e^{-i\lambda(T-\tau)} e^{-\lambda\tau(i-1)} (1 - e^{-\lambda\tau})$ , which converges to  $\frac{1 - e^{-\lambda\tau}}{1 - e^{-\lambda T}}$ . The probability that it takes two contacts before detecting the next one (i.e.,  $\mathbb{P}(N^* = 2)$ ) can be computed, again considering all intervals  $i$  in which the contact can be detected, as the probability that only one contact occurs in the OFF intervals before the  $i$ -th ON times the probability that zero contacts occur in the ON intervals before the  $i$ -th times the probability that a contact occurred in the  $i$ -th ON interval. This corresponds to  $\mathbb{P}(N^* = 2) = \sum_{i=1}^{\infty} i\lambda(T - \tau) e^{\lambda(T-\tau)i} e^{-\lambda\tau(i-1)} (1 - e^{-\lambda\tau})$ , which converges to  $\lambda(T - \tau)(e^{\lambda\tau} - 1) Li_{-1}(e^{-\lambda T})$ . Generalising to the case  $N^* = k$ , we obtain Equation A.12.

So far, we have focused on what happens after the last contact in an ON interval. We now consider what happens before that last contact, i.e., how large is the burst of contacts in the ON interval. Again, we can exploit the property of Poisson Point Processes discussed above, so the number  $N_{ON}$  of contacts in an ON interval is distributed as  $\text{Poisson}(\lambda\tau)$ . Each contact in the burst accounts for one sample of  $N = 1$ , except the last one (which is modelled by  $N^*$ ). Thus, the first  $n - 1$  contacts of a burst weight  $\frac{\sum_{n=1}^{\infty} (n-1) \mathbb{P}(N_{ON}=n)}{\sum_{n=1}^{\infty} n \mathbb{P}(N_{ON}=n)}$  in the distribution of  $N$ . This

expression simplifies to  $\frac{\lambda\tau - (1 - e^{-\lambda\tau})}{\lambda\tau}$ . Hence, we can write the relation  $N = \begin{cases} 1 & \frac{\lambda\tau - (1 - e^{-\lambda\tau})}{\lambda\tau} \\ N^* & \frac{(1 - e^{-\lambda\tau})}{\lambda\tau} \end{cases}$ , from which we obtain the PMF of  $N$  in Equation A.11.  $\square$

From the expression in Equation A.11 we can derive the tail behaviour of the PMF of  $N$ . In particular, exploiting the well-known result  $\lim_{Re(s) \rightarrow -\infty} Li_s(e^\mu) = \Gamma(1 - s)(-\mu)^{s-1}$ , we obtain that  $\mathbb{P}(N = k)$  decays as  $(\frac{T-\tau}{T})^{k-1}$  for large  $k$ , i.e., exactly as predicted by the Geometric approximation.

## A.7 Proof of Lemma 5

We focus on the squared coefficient of variation of  $\tilde{S}$ . Specifically, we know that  $cv_{\tilde{S}}^2 = \frac{cv_S^2}{\mathbb{E}[N]} + cv_N^2$ , so, in order for  $\tilde{S}$  to show a hyper-exponential behaviour, quantity  $\frac{cv_S^2}{\mathbb{E}[N]} + cv_N^2$  has to be greater

than 1. If we rewrite this expression as a function of  $g$  and  $p$ , we obtain the following:

$$cv_S^2 > 1 - \frac{2g}{p} + \frac{2}{1-g+p}. \quad (\text{A.13})$$

We call the right-hand side of this inequality  $\xi(g, p)$ , thus  $\xi(g, p) = 1 - \frac{2g}{p} + \frac{2}{1-g+p}$ . In Figure A3

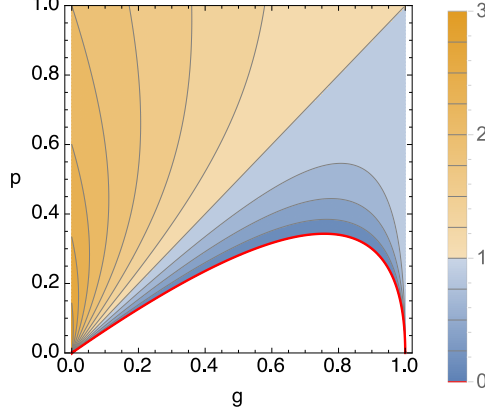

Figure A3: Hypoexponential/hyperexponential regions depending on  $cv_S^2, g, p$

we plot  $\xi(g, p)$ . We color in blue the regions where  $\xi(g, p)$  is smaller than 1, in orange the regions where  $\xi(g, p)$  is greater than 1. Let us first focus on case  $cv_S^2 \geq 1$ . When  $g \geq p$ ,  $\xi(g, p)$  is always smaller than 1, hence for any  $cv_S^2 > 1$ , the inequality in Equation A.13 is always satisfied, thus leading to a hyper-exponential detected intercontact time  $\tilde{S}$ . When  $p > g$ ,  $\xi(g, p) > 1$ , thus the squared coefficient of variation of  $\tilde{S}$  depends on whether  $cv_S^2$  stays above or below  $\xi(g, p)$ . When it stays below (inequality in Equation A.13 not satisfied), we get the interesting case of a hypo-exponential detected intercontact time obtained starting from a hyper-exponential one. Since  $\xi(g, p) < 3$  for all  $g, p$ , when  $cv_S^2 > 3$  the inequality in Equation A.13 is always satisfied and only an hyper-exponential behaviour for  $\tilde{S}$  is possible.

Let us now focus on case  $0 < cv_S^2 \leq 1$ . When  $p \geq g$ , the detected intercontact time can only be hypo-exponential, because  $\xi(g, p) > 1$  while  $cv_S^2 < 1$ . Vice versa, denoting with  $\omega(g) = \frac{3}{2}(g - 1) + \frac{1}{2}\sqrt{9 - 10g + g^2}$  the function (plotted in red in Figure A3) resulting from the intersection between when  $\xi(g, p)$  and plane  $cv_S^2 = 0$  (hence  $\xi(g, p) < 0$  for  $p < \omega(g)$ ), we get that  $\tilde{S}$  will always be hyper-exponential for  $p < \omega(g)$ , because the inequality in Equation A.13 is always satisfied. For the values in between, one has to evaluate whether  $cv_S^2$  stays above or below the surface  $\xi(g, p)$ .

## B Proofs for Section 4 (non-negligible contact duration case)

### B.1 Proof of Lemma 8

Consider a detected contact. The overlap between the CONTACT state of the contact process and the ON state of the joint duty cycle can happen in two ways: either the contact starts in an ON interval or it starts in an OFF interval and lasts until the next ON interval. In the latter case, we do not observe the same contact distribution as that of  $C_i$ , since only contacts lasting until the next ON interval can be considered. Instead, we observe a contact of length  $C_i^{hit}$ , which can be derived as the distribution of  $C_i$  knowing that  $Z^{OFF} + C_i > T - \tau$ , i.e.,  $f_{C_i^{hit}}(c) = \mathbb{P}(C_i = c | C_i + Z^{OFF} > T - \tau)$ , which becomes Equation 13. Based on the observation above, a detected contact can be distributed as  $C_i$  or  $C_i^{hit}$ . For convenience of notation, we drop subscript  $i$ , since the actual sequence number of the contact is not important. When the contact happens in

an ON interval, its starting point is  $T - \tau + Z^{ON}$ .  $H$  takes value 1 (i.e. the contact overlaps with just one ON interval) if  $T - \tau + Z^{ON} + C$  ends before  $2T - \tau$ , it takes value 2 if  $T - \tau + Z^{ON} + C$  ends between  $2T - \tau$  and  $3T - \tau$ , and so on. When the detected contact happens in an OFF interval, its starting point is  $Z^{OFF}$ , hence  $H$  is equal to 1 when  $Z^{OFF} + C^{hit}$  is smaller than  $2T - \tau$ ,  $H$  is equal to 2 when  $Z^{OFF} + C^{hit}$  is in  $[2T - \tau, 3T - \tau)$ , etc. This discussion can be cast into the following equations, taking also into account the slight difference between case  $H = 1$  and all others (basically, in the former there is no lower bound to be considered since the contact may begin and end in the same ON interval).

$$\mathbb{P}\{H = 1\} = p_s^{ON} \mathbb{P}(T - \tau + Z^{ON} + C < 2T - \tau) + p^{OFF} \mathbb{P}(Z^{OFF} + C^{hit} < 2T - \tau),$$

$$\begin{aligned} \mathbb{P}\{H = h\} = & p_s^{ON} \mathbb{P}(hT - \tau < T - \tau + Z^{ON} + C < (h+1)T - \tau) + \\ & + p_s^{OFF} \mathbb{P}(hT - \tau < Z^{OFF} + C^{hit} < (h+1)T - \tau), \quad \forall h > 1. \end{aligned}$$

Then, after simple computation, we get Equation 12.

## B.2 Proof of Theorem 2

A measured contact cannot last, by definition, more than  $\tau$  seconds, which is the maximum length of an uninterrupted (by an OFF interval) stretch of contact. More specifically, a measured contact is the result of the tagged pair of nodes being at once in contact with each other and in the ON interval of their duty cycle. So, for deriving the measured contact we first have to understand how the contact and the ON intervals overlap. Then, for each overlap, we derive i) the probability that it takes place, and ii) the shape of the measured contact in this case.

The simplest case, which we study first, is when the contact overlaps with just one ON interval of the duty cycle, case corresponding to  $H = 1$ . Case  $H = 1$  is a special case in our derivation, as it will become clear in the following. As illustrated in Figure 8, when  $H = 1$  there are four different types of overlapping depending on whether the contact starts in either an ON or OFF interval and whether it ends in either an ON or OFF interval. The probability that a contact starts in an ON or OFF interval is given by Lemma 7. Deriving the probability of a contact ending in an ON or OFF interval is slightly more complicated, because, for  $H = 1$  we don't want to rely on the slowly varying assumption for  $C_i$  (i.e., we don't want to exploit Corollary 4). Depending on whether the contact starts in ON/OFF we can derive the time at which it ends as  $Y^{ON} = Z^{ON} + C$  or  $Y^{OFF} = Z^{OFF} + C$ . Quantities  $Y^{ON}$  and  $Y^{OFF}$  can be obtained using the standard formula for the sum of random variables [4]. When  $H = 1$ , we also know that they are constrained to be smaller than  $2T - \tau$  (otherwise the contact would span two ON intervals and  $H$  could not be equal to 1). Thus, when the contact starts in an ON interval, we can shift the time axis by  $T - \tau$  and compute the probability that the contact ends in the same ON interval as  $\mathbb{P}(Y^{ON} < \tau) / \mathbb{P}(Y^{ON} < T)$ . The probability that the contact ends in an OFF interval can be obtained as one minus this probability. Taking Figure 8 as reference, the probability associated with cases (a) and (c) can thus be computed as  $\frac{\tau}{T} \cdot \mathbb{P}(Y^{ON} < \tau) / \mathbb{P}(Y^{ON} < T)$  and  $\frac{\tau}{T} \cdot [1 - \mathbb{P}(Y^{ON} < \tau) / \mathbb{P}(Y^{ON} < T)]$ , respectively. A similar line of reasoning can be followed for the other two cases. In fact, the probability that the contact starts in an OFF interval is given by  $\frac{T-\tau}{T}$ . Knowing that the contact started in an OFF interval, the contact can either end in the next ON interval or in the following OFF interval. The probability of the former can be obtained as  $\mathbb{P}(T - \tau < Y^{OFF} < T) / \mathbb{P}(T - \tau < Y^{OFF} < 2T - \tau)$ , the probability of the latter as its complement. Hence, the probability of case (b) and case (d) is  $\frac{T-\tau}{T} \cdot \mathbb{P}(T - \tau < Y^{OFF} < T) / \mathbb{P}(T - \tau < Y^{OFF} < 2T - \tau)$  and  $\frac{T-\tau}{T} \cdot [1 - \mathbb{P}(T - \tau < Y^{OFF} < T) / \mathbb{P}(T - \tau < Y^{OFF} < 2T - \tau)]$ , respectively.

Now that we can quantify the probability that each type of overlapping takes place, we move to studying the length of the measured contact duration for each of these combinations. In case (a) of Figure 8, the contact is fully contained in the ON interval, and the measured contact duration is equal to the duration of  $C$  knowing that the sum  $Y^{ON} = Z^{ON} + C$  belongs to the ON interval. We denote this quantity as  $C^{short}$ . Its density can be derived as  $f_{C^{short}}(c) = \mathbb{P}(C = c | C + Z^{ON} < \tau)$ , defined for  $x \in (0, \tau]$ . After applying the law of conditional probability and taking into account

the constraint  $C + Z^{ON} < \tau$ , we obtain  $f_{C_{short}}(c) = \int_0^{\tau-c} \frac{\mathbb{P}(C=c)}{\mathbb{P}(C < \tau-z)} \mathbb{P}(Z^{ON} = z) dz$ . Replacing  $\mathbb{P}(Z^{ON} = z)$  with  $\frac{\tau}{T}$  (Lemma 7) and operating a change of variable ( $u = \tau - z$ ) we obtain Equation 15. In case (b) of Figure 8, the measured contact is equal to  $\tau$  (it lasts for the whole ON interval). In case (c), the measured contact is equal to  $\tau - Z^{ON}$ , which is distributed as  $Z^{ON}$ . Finally, if the detected contact starts in the OFF interval and ends in the ON interval (corresponding to case (d) in the figure) the measured contact lasts as long as  $Y^{OFF}$  truncated in  $[T - \tau, T]$  and shifted by  $T - \tau$ . We refer to this quantity as  $C^{res}$ . Leveraging the formulas for truncated and shifted random variables [4], the distribution of  $C_{res}$  can be obtained as shown in Equation 16. This concludes the derivations for case  $H = 1$ .

We now study what happens when  $H = 2$ . Again, first we study the possible ways the contact and the ON intervals overlap, then we characterise the measured contact in each of these cases. When  $H = 2$  the contact begins in  $[0, T]$  and ends in  $[2T - \tau, 3T - \tau]$  (see Figure B4). Two separate measured contacts are introduced: one (totally or partially) overlapping with the first ON interval and one (totally or partially) overlapping with the second ON interval. Initially, we focus on the one overlapping with the first ON interval. As illustrated in Figure B4, there are two cases. With probability  $\frac{\tau}{T}$  (i.e., when the real contact starts in an ON interval) we observe a measured contact time like the one in Figure 8(c), whose length we had found to be equal to  $Z^{ON}$ . With probability  $\frac{T-\tau}{T}$  (i.e., when the real contact starts in an OFF interval), we observe  $\tau$ . Let us now focus on the second measured contact, i.e., on the portion of the real contact that overlaps with the second ON interval. This measured contact starts being detected at  $2T - \tau$  but it can stop either in the same ON interval or in the following OFF interval. The probabilities of these two events depend on  $C$  and on the interval  $[2T - \tau, 2T]$ . More in general, if  $H = h$ , whether a real contact ends in ON or OFF depends on  $C$  and on the interval  $[hT - \tau, hT]$ . In order to simplify the derivations, we assume that  $C$  is slowly varying in intervals of type  $[hT - \tau, hT]$  with  $h > 1$ . With this assumption we can exploit Corollary 3, so the end of a contact becomes uniformly distributed in the interval in which it takes place. Hence, the probability of a contact ending in an ON or OFF interval does not depend anymore on  $H$  or on the specific distribution of  $C$ , and it is simply given by  $\frac{\tau}{T}$  and  $\frac{T-\tau}{T}$  respectively. We now characterise the measured contact in these two cases. As illustrated in Figure B4, the measured contact is equal to  $\tau$  if the contact ends in an OFF interval (probability:  $\frac{T-\tau}{T}$ ). When the contact ends in an ON interval, instead, the measured contact is equal to  $Z^{ON}$ , which follows directly from the slowly varying approximation for  $C$  (Corollary 3). Summarising, when  $H = 2$  and assuming that  $C$  is slowly varying in  $[2T - \tau, 2T]$ , the measured contact times that we observe can be either  $\tau$  or  $Z^{ON}$ . The probability that we observe  $Z^{ON}$  is equal to  $2\frac{\tau}{T}$ , which is the sum of the probability  $\frac{\tau}{T}$  that we observe  $Z^{ON}$  at the first intersection with an ON interval and the probability  $\frac{\tau}{T}$  that we observe  $Z^{ON}$  at the second intersection with an ON interval. Vice versa, the probability that we observe  $\tau$  is equal to  $2\frac{T-\tau}{T}$ , which can be computed following a similar line of reasoning.

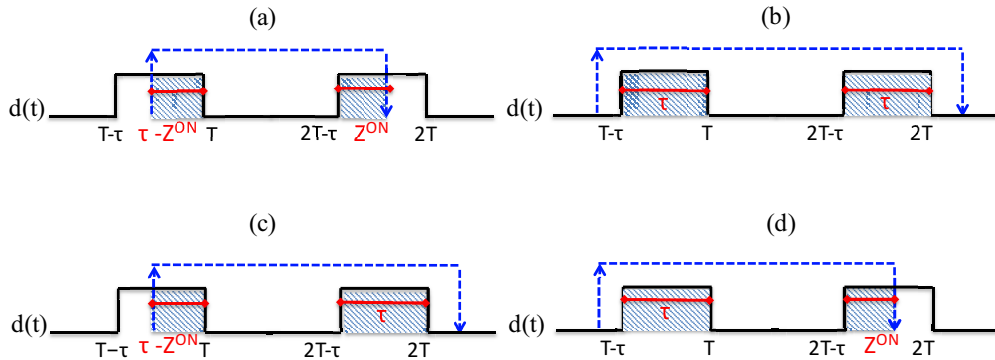

Figure B4: Case  $H = 2$ : types of overlapping.

More generally, when  $H = h$ ,  $h$  measured contacts are introduced. It is easy to see that the first and last of these contacts correspond to those that we have observed also for  $H = 2$ . Instead, the  $h - 2$  intermediate ones are all equal to  $\tau$  because the original contact completely overlaps

with the  $h - 2$  ON intervals between the first and the  $h$ -th one. Summarising, the detected contact can be equal to one of  $\{\tau, Z^{ON}, C^{short}, C^{res}\}$  when  $H = 1$  and to one of  $\{\tau, Z^{ON}\}$  when  $H \geq 2$ . Weighting each case with the actual probability of occurrence (which we have already discussed in this proof) we obtain Equation 14.

### B.3 Proof of Theorem 9

When nodes refrain from entering the low-power state once they detect a contact, deriving the distribution of  $\tilde{C}$  is easier than in Theorem 2. In fact, in this case, the original contact is modified only if the contact starts in an OFF interval, i.e., with probability  $\frac{T-\tau}{T}$ . Otherwise, with probability  $\frac{\tau}{T}$ ,  $\tilde{C}$  is distributed as  $C$ .

When the contact starts in an OFF interval, the initial part of the contact is lost. In this case  $\tilde{C}$  is distributed as  $C^{res*}$ , i.e., as  $Y^{OFF}$  constrained to outlive the OFF interval minus the length of the OFF interval itself. This corresponds to the expression for  $C^{res*}$  in Equation 18.

### B.4 Proof of Theorem 3

We have already explained how to derive the two components of the mixture distribution for  $\tilde{S}$  in the main text. The only missing part is the derivation of the probability with which each component is taken. Recall that there are two types of measured intercontact times: real ones and pseudo. One element of the first type is introduced any time a measured contact ends. Instead,  $H - 1$  elements of the second type are introduced by each detected contact spanning  $h$  ON intervals. Thus, elements of the first type weight one for any  $H$  value, while elements of the second type weight more (specifically,  $H - 1$ ). After taking into account the probability distribution of  $H$  from Lemma 8, Equation 20 follows.

### B.5 Proof of Lemma 10

When deriving the distribution of  $N$ , Equation 1 still holds also in the case of non-negligible contact duration. So, again,  $\mathbb{P}(N = k) = \mathbb{P}(E_1 = 0, \dots, E_{k-1} = 0, E_k = 1)$ , where  $E_k$  is zero if the  $k$ -th contact goes undetected, one otherwise. Again, note that  $E_k$  is dependent on the outcome of all previous events  $E_1, \dots, E_{k-1}$ .

Let us start from the analysis of case  $N = 1$ , corresponding to the first contact being detected. For the sake of convenience, we focus on the complementary event, i.e., first contact not detected. This can happen only when the first contact starts in an OFF interval and ends before the beginning of the next ON interval. Recalling that  $X_i$  and  $Y_i$  denote the start and end point, respectively, of the  $i$ -th contact, this is equivalent to:

$$\mathbb{P}(N = 1) = 1 - \sum_{n_1=2}^{\infty} \mathbb{P}(X_1 \in \mathcal{I}_{n_1}^{OFF}, Y_1 \in \mathcal{I}_{n_1}^{OFF}) \quad (\text{B.14})$$

$$= 1 - \sum_{n_1=2}^{\infty} \mathbb{P}(Z + S \in \mathcal{I}_{n_1}^{OFF}) \mathbb{P}(Z^{OFF} + C < T - \tau) \quad (\text{B.15})$$

where the second equality follows after approximating (Lemma 6 and Corollary 3) the displacement of start/end points of contacts as uniformly distributed in the intervals in which they take place. In the following, we will denote the above quantity as  $\hat{g}$ , similarly to the non-negligible contact case.

Now we move to  $N = 2$ , which implies that the first contact is not detected while the second one is. The probability of the first contact not being detected is equivalent to the complementary probability that we have derived above. The probability that the second contact is detected is similar to the probability of the first contact being detected with the difference that in this case

we know for sure that the first contact was fully contained in an OFF interval.

$$\begin{aligned}\mathbb{P}(N=2) &= \sum_{n_1=2}^{\infty} \mathbb{P}(X_1 \in \mathcal{I}_{n_1}^{OFF}, Y_1 \in \mathcal{I}_{n_1}^{OFF}) \left[ 1 - \sum_{n_2=n_1+1}^{\infty} \mathbb{P}(X_2 \in \mathcal{I}_{n_2}^{OFF}, Y_2 \in \mathcal{I}_{n_2}^{OFF}) \right] \\ &= (1-\hat{g}) \left[ 1 - \sum_{n_2=2}^{\infty} \mathbb{P}(Z^{OFF} + S \in \mathcal{I}_{n_2}^{OFF}) \mathbb{P}(Z^{OFF} + C < T - \tau) \right]\end{aligned}\quad (\text{B.16})$$

Similarly to the negligible contact case, we denote the quantity in square brackets above as  $\hat{p}$ .

Let us now consider case  $N=3$ , corresponding to the first two contacts missed and the third one detected. The probability that the first contact is missed has been computed above and it is given by  $1-\hat{g}$ . The probability that the second contact is missed is simply the complementary probability that the contact is detected, i.e.  $1-\hat{p}$ . Finally, it is easy to see that the probability of detecting the third contact is again given by  $\hat{p}$ . Generalising, we obtain the same expression for the PMF of  $N$  as in Theorem 1, with the difference that  $g$  and  $p$  are computed differently from  $\hat{g}$  and  $\hat{p}$ .

## C Further results for the trace-based validation in Section 4.4

Table 1: Summary of most popular contact datasets.

| Dataset               | Technology | Duration [days] | Participants | T [s] |
|-----------------------|------------|-----------------|--------------|-------|
| Cambridge (HAGGLE)    | Bluetooth  | 3               | 12           | 120   |
| Infocom 2005 (HAGGLE) | Bluetooth  | 4               | 41           | 120   |
| Infocom 2006 (HAGGLE) | Bluetooth  | 4               | 70           | 120   |
| Rollernet (UPMC)      | Bluetooth  | 1               | 62           | 15    |
| Reality Mining (MIT)  | Bluetooth  | 16              | 246          | 300   |
| PMTR (UniMi)          | Custom     | 19              | 44           | 1     |

### C.1 Analysis of the PMTR and RollerNet datasets (Section 4.4)

Tables 2 and 3 summarise the results of our analysis of the PMTR and RollerNet contact traces.

Table 2: Exponential contact and intercontact times hypothesis. Rates for contact ( $\mu$ ) and intercontact ( $\lambda$ ) times are estimated using MLE fitting. The third column contains the percentage of pairs with more than 9 samples. The fourth column contains the percentage of pairs that pass the Cramér-Von Mises test (pairs with less than 9 samples are excluded).

| Type            | Dataset   | Included | CvM    | Min.      | 1st Qu.   | Median    | Mean      | 3rd Qu.   | Max.      |
|-----------------|-----------|----------|--------|-----------|-----------|-----------|-----------|-----------|-----------|
| CT - $\mu$      | pmtr      | 40.06%   | 36.94% | 0.0000714 | 0.005448  | 0.01253   | 0.01794   | 0.01873   | 0.4118    |
| CT - $\mu$      | rollernet | 43.95%   | 75.33% | 0.01692   | 0.03979   | 0.04921   | 0.05229   | 0.06034   | 0.13850   |
| ICT - $\lambda$ | pmtr      | 37.74%   | 4.76%  | 6.910e-06 | 1.132e-05 | 3.732e-05 | 5.017e-04 | 6.575e-04 | 3.127e-03 |
| ICT - $\lambda$ | rollernet | 84.88%   | 35.76% | 0.0007926 | 0.001727  | 0.0025580 | 0.003082  | 0.00384   | 0.0184    |

### C.2 Analysis of the Infocom’05 and Reality Mining datasets

The discussion in Section 4.4 has focused on the PMTR and RollerNet traces because, thanks to their short duty cycle, they are expected to be closer to real-life contact and intercontact times. However, in the literature other traces are typically more popular than the PMTR and RollerNet ones. From Table 1 probably the most widely used traces are the Infocom 2005 [8] and the Reality Mining [5] traces. In the following, for these traces we carry out the same study that we performed earlier for the PMTR and RollerNet traces, in order to understand whether their contact and intercontact times vary in ranges for which our model provides accurate estimates.

Table 3: Pareto contact and intercontact times hypothesis. Pareto parameters  $(\alpha, b)$  are estimated using MLE fitting. The third column contains the percentage of pairs with more than 9 samples. The fourth column contains the percentage of pairs that pass the Cramér-Von Mises test (pairs with less than 9 samples are excluded).

| Type           | Dataset   | Included | CvM    | Min.  | 1st Qu. | Median | Mean   | 3rd Qu. | Max.     |
|----------------|-----------|----------|--------|-------|---------|--------|--------|---------|----------|
| CT - $\alpha$  | pmtr      | 40.06%   | 99.21% | 1.412 | 1.554   | 1.754  | 1.898  | 2.097   | 3.250    |
| CT - $b$       |           |          |        | 3.00  | 19.00   | 43.00  | 245.40 | 91.25   | 13070    |
| CT - $\alpha$  | rollernet | 43.95%   | 98.79% | 1.444 | 2.348   | 2.695  | 2.667  | 3.042   | 3.386    |
| CT - $b$       |           |          |        | 2.00  | 11.00   | 12.00  | 13.68  | 15.00   | 53.00    |
| ICT - $\alpha$ | pmtr      | 37.74%   | 97.48% | 1.33  | 1.458   | 1.481  | 1.562  | 1.553   | 3.00     |
| ICT - $b$      |           |          |        | 69.00 | 586.8   | 1326.0 | 7991.0 | 2910.0  | 172900.0 |
| ICT - $\alpha$ | rollernet | 84.88%   | 98.94% | 1.400 | 1.579   | 1.736  | 1.906  | 2.091   | 3.500    |
| ICT - $b$      |           |          |        | 16.00 | 20.00   | 28.00  | 120.7  | 169.5   | 1341.0   |

First of all, we filter out those pairs for which we have less than 9 samples. The percentage of pairs that are left after this pruning are reported in Table 4. Note that, for the Reality Mining experiment, there are much more participants than in other traces (Table 1) but for many of the pairs the number of collected contact samples is low. Next, we apply the fitting technique described in Section 4.4 and we run the Cramér-von Mises test for the exponential hypothesis (Table 5) and the Pareto hypothesis (Table 6). The procedure from [3] for the automatic derivation of  $b$  was not able to yield results for the Reality Mining trace, hence we manually set  $b$  equal to the duty cycling period and we only estimated the  $\alpha$  values.

Table 4: Node pairs for which enough samples are available.

| Type | Infocom | Reality |
|------|---------|---------|
| CT   | 60.49%  | 22.09%  |
| ICT  | 81.83%  | 29.88%  |

Table 5: Exponential contact and intercontact times hypothesis. Rates for contact ( $\mu$ ) and intercontact ( $\lambda$ ) times are estimated using MLE fitting. Only pairs with more than 9 samples are considered. The third column contains the percentage of pairs that pass the Cramér-Von Mises test.

| Type            | Dataset | CvM    | Min.      | 1st Qu.   | Median    | Mean      | 3rd Qu.   | Max.      |
|-----------------|---------|--------|-----------|-----------|-----------|-----------|-----------|-----------|
| CT - $\mu$      | infocom | 87.90% | 0.0006848 | 0.0021150 | 0.0030240 | 0.0032580 | 0.0041280 | 0.0094210 |
| CT - $\mu$      | reality | 85.32% | 0.0000673 | 0.0002903 | 0.0004163 | 0.0004777 | 0.0005889 | 0.0020900 |
| ICT - $\lambda$ | infocom | 3.42%  | 3.002e-05 | 4.976e-05 | 6.930e-05 | 2.622e-04 | 2.643e-04 | 1.537e-03 |
| ICT - $\lambda$ | reality | 23.08% | 2.145e-07 | 8.736e-07 | 1.268e-06 | 1.753e-06 | 1.995e-06 | 1.478e-05 |

In order to better understand how the Infocom and Reality Mining fitting results compare to those obtained from the PMTR and RollerNet traces – which, we recall, have a much shorter duty cycling period – we plot the CDF of the exponential and Pareto parameters obtained with the fitting procedures (only for those pairs that pass the Cramér-von Mises test). The results are shown in Figures C5 and C6. Let us start with the exponential case. Recall that in Section 4.4 we compare simulation results and model predictions for significant points of the rate distributions corresponding to the minimum and maximum values, first and third quartiles, median and mean. From the slowly varying condition we know that greater rate values are more challenging in order to satisfy  $\lambda T \ll 1$  (for intercontact times) or  $\mu T \ll 1$  (for contact duration). Figures C5 and C6 show that the RollerNet trace features the highest rates for both the contact and intercontact times. Hence, if our theoretical model is accurate across the rate values of the RollerNet trace, it will be accurate also for the other traces (the duty cycling process being equal). In particular, the Reality Mining dataset is the less challenging from this standpoint, as it features the smallest rates among all four traces. Next, we consider the Pareto contact and intercontact times assumptions. Figures C5 and C6 show that, for contact and intercontact times, the smaller  $b$  values are achieved for the RollerNet trace. Thus, recalling that for larger

Table 6: Pareto contact and intercontact times hypothesis. Pareto parameters  $(\alpha, b)$  are estimated using MLE fitting. Only pairs with more than 9 samples are considered. The third column contains the percentage of pairs that pass the Cramér-Von Mises test.

| Type           | Dataset | CvM    | Min.  | 1st Qu. | Median | Mean   | 3rd Qu. | Max.    |
|----------------|---------|--------|-------|---------|--------|--------|---------|---------|
| CT - $\alpha$  | infocom | 98.39% | 1.417 | 1.825   | 2.085  | 2.177  | 2.469   | 3.273   |
| CT - $b$       |         |        | 2.0   | 117.0   | 128.0  | 239.6  | 244.2   | 8672.0  |
| CT - $\alpha$  | reality | 91.10% | 1.444 | 1.958   | 2.458  | 2.490  | 3.059   | 3.500   |
| CT - $b$       |         |        | 191.0 | 646.5   | 1566.0 | 2264.0 | 3449.0  | 23640.0 |
| ICT - $\alpha$ | infocom | 99.25% | 1.375 | 1.467   | 1.496  | 1.543  | 1.573   | 2.470   |
| ICT - $b$      |         |        | 121.0 | 147.0   | 235.0  | 1005.0 | 528.2   | 28800.0 |
| ICT - $\alpha$ | reality | 14.36% | 1.133 | 1.173   | 1.199  | 1.203  | 1.227   | 1.364   |
| ICT - $b$      |         |        | 300   | 300     | 300    | 300    | 300     | 300     |

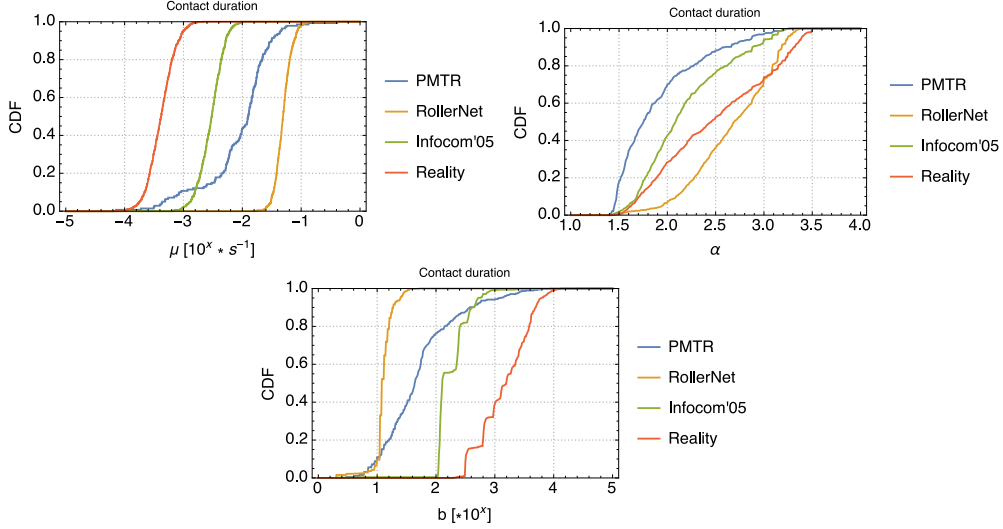

Figure C5: Contact duration: comparison of parameters across different traces

$b$  values the model yields better predictions, Figures C5 and C6 indicate that model predictions will be generally better for the Infocom and Reality Mining traces also in the Pareto case.

The main finding of this analysis is that the Reality Mining and Infocom datasets are actually less challenging for our model than the PMTR and RollerNet traces. This is due to the fact that, with their parameters, the slowly varying condition is achieved more easily (the duty cycling process being the same), and thus the approximations introduced by our model impact negligibly on the results.

### C.3 Further results for the validation in Section 4.4.1

Figure C7 shows how the contribution of the different components to the mixture  $\tilde{C}$  varies with  $\mu$ . When  $\mu$  is large (i.e. when contact duration is short) all contributions to  $\tilde{C}$  are negligible except for  $C^{res}$  and  $C^{short}$ . In fact, with short contacts, a measured contact corresponds to either a contact fully contained in an ON interval or to one that started in OFF and then lasted until an ON (but since the contact is short, it rarely lasts beyond the ON interval in which it is detected). Vice versa, when  $\mu$  is very small (i.e. when contacts are very long), the major component of  $\tilde{C}$  is  $\tau$ , since this long contact is split into many shorter contacts.

While Figure C7 helps us understand the interplay between the different components in  $\tilde{C}$ , we have yet to investigate the quality of the predictions provided by Theorem 2. The situation here is partially different than from what we discussed for the intercontact times in the negligible contact

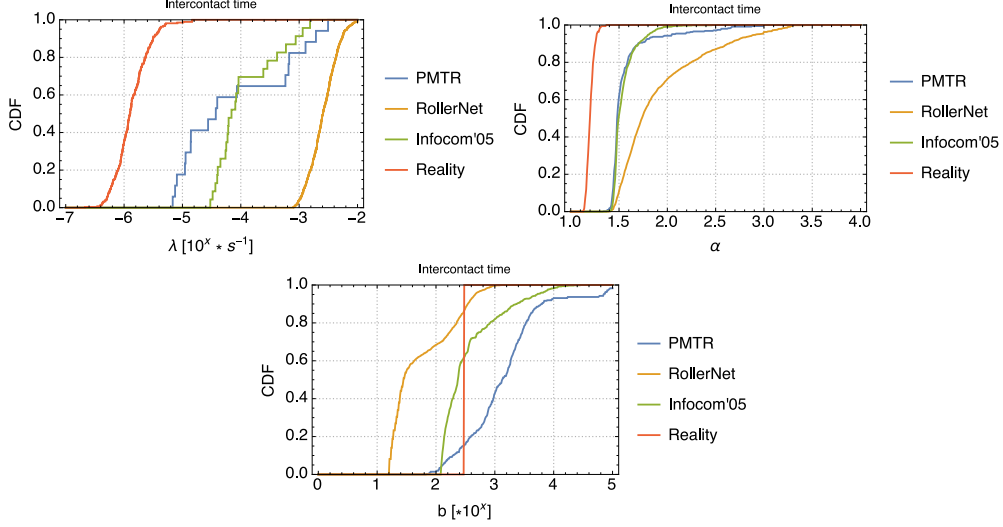

Figure C6: Intercontact times: comparison of parameters across different traces

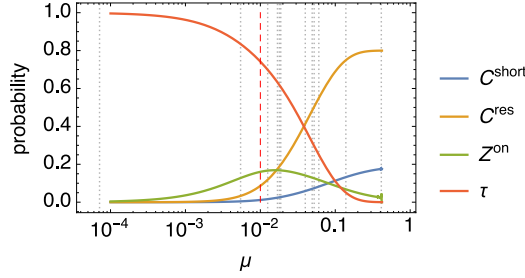

Figure C7: Interplay between the different components of  $\tilde{C}$ . The grey vertical lines correspond to significant values of the PMTR and RollerNet rates (min, 1st quart., median, mean, 3rd quart., max).

case (Section 3.3). In the latter case, predictions were as good as intercontact times were slowly varying in ON/OFF intervals. Here, the slowly varying property of  $C_i$  (which can be assessed using the sufficient condition  $\mu T \ll 1$ , similarly to what we have done so far for intercontact times) is again a predictor of the accuracy of Theorem 2, but it is not the only element. In fact, in Theorem 2 we did not use the slowly varying property for case  $H = 1$ , hence, if the probability of  $H = 1$  is very high, the predictions of Theorem 2 will be good regardless of  $C_i$  being slowly varying or not. The probability of  $H = 1$  (Lemma 8) only depends on  $\mu$  once  $\tau$  and  $T$  have been fixed, and it is plotted in Figure C8. Under our  $\tau = 20s, T = 100s$  configuration, we observe that soon after  $\mu = 10^{-2}$ ,  $H = 1$  becomes the predominant component in the distribution.  $\mu = 10^{-2}$  is also the upper limit to  $C_i$  being slowly varying (in fact,  $10^{-2} \cdot 100 = 1$ ). Hence, we expect discrepancies between the predictions of Theorem 2 and simulation results when  $\mu$  is in the neighbourhood of  $10^{-2}$ . In fact, around  $\mu = 10^{-2}$  we are in a situation such that the dominance of  $H = 1$  has yet to kick in while at the same time the slowly varying approximation does not hold.

#### C.4 Further results for the validation in Section 4.4.2

In order to complement the results discussed in Section 4.4.2, here we provide a general analysis of the dependence of  $\tilde{C}$  on the Pareto parameters  $\alpha$  and  $b$ , and on  $\mathbb{P}(H = 1)$ , similarly to what we have done in Figures C7 and C8. To this aim, we first need to make sure that  $H$  in the Pareto case does not suffer from the convergence problems that afflict heavy-tailed distribution depending on

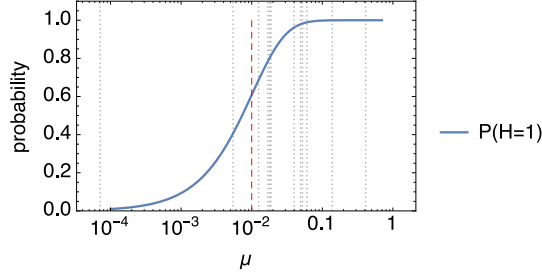

Figure C8: Weight of the  $H = 1$  component. The red line corresponds to  $\mu = 1/T$ , the grey vertical lines correspond to PMTR and RollerNet rates (min, 1st quart., meadian, mean, 3rd quart., max).

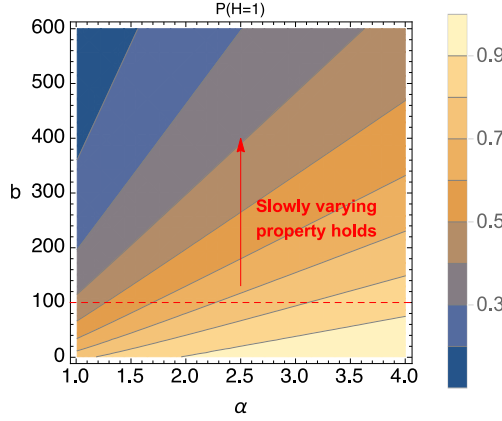

Figure C9: How  $P(H = 1)$  varies as a function of  $\alpha, b$ .

the value of their exponent. Based on Lemma 8, it is easy to show that the CCDF of  $H$  decays as  $\frac{1}{x^\alpha}$ , hence its expectation does not converge [1] for values of  $\alpha$  smaller than 1. Similarly to what happens with the delay, the non-negligible presence of arbitrarily large intercontact times steers the network towards a degenerate behavior. However, in our two reference datasets, all parameters  $\alpha$  are greater than 1, so convergence problems do not show up in our case.

Next, we consider the predominance of the different components of  $H$ . When  $H \geq 2$ , our model in Theorem 2 relies on the slowly varying approximation for the contact distribution, hence it may introduce errors when the slowly varying hypothesis does not hold for  $C_i$ . When  $H = 1$ , this assumption is not exploited, hence predictions are expected to be accurate regardless of  $C_i$  being slowly varying or not. In Figure C9 we plot how  $P(H = 1)$  varies as a function of  $\alpha$  and  $b$ . When  $P(H = 1)$  is high, predictions will be accurate. Otherwise, we need to rely on the sufficient condition for a Pareto distribution to be slowly varying. Based on Figure C9, we observe that the only region in which theoretical predictions are expected to be less accurate corresponds to the bottom left one. In fact, for  $b \gg T$  ( $b = T$  is indicated by the dashed red line in the figure) the slowly varying property holds, hence accuracy is guaranteed. When  $b < T$ , the model is expected to predict accurately when  $P(H = 1)$  is high, which is generally true for  $\alpha > 2$  according to Figure C9.

We now analyse the interplay between the different components of  $\tilde{C}$  as we vary  $\alpha$  and  $b$ . In Figure 10(a) we vary  $\alpha$  and we fix  $b$  to three representative values (min, mean, max of the PMTR trace). We observe that there are two components ( $\tau$  and  $Z_{on}$ ) that take turns in dominating  $\tilde{C}$  as  $\alpha$  increases, but only when  $b$  is small (lefthand side figure). For larger value of  $b$  the effect of increasing values of  $\alpha$  goes from small to negligible. For what concerns the effect of  $b$  on  $\tilde{C}$ , we observe in Figure 10(b) that variations of  $b$  have generally a significant effect. The trend is

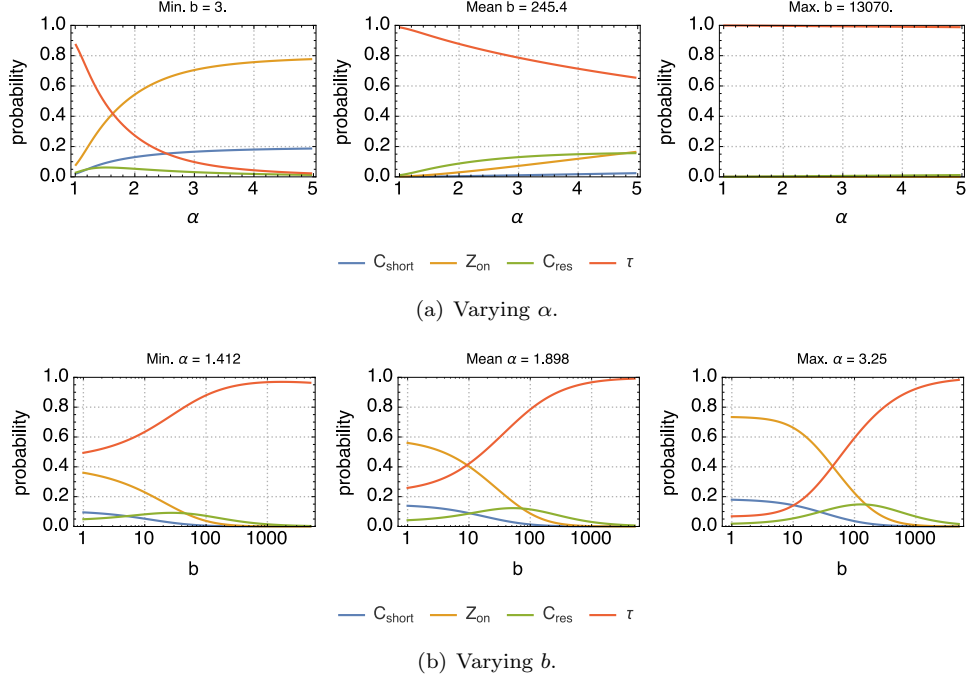

Figure C10: Interplay between the different components of  $\tilde{C}$ .

clear: when  $b$  is small contact times tend to be shorter, hence we observe fewer  $\tau$  components. Vice versa, when  $b$  is large, the  $\tau$  component dominates in  $\tilde{C}$ .

## D Proofs for Section 5

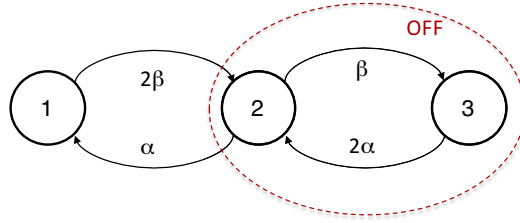

Figure D11: Continuous Time Markov Chain for the stochastic duty cycling.

As discussed in Section 5, we model the states of our system using a Continuous Time Markov Chain (CTMC) with three states (Figure D11). In state (1) both nodes are ON, in state (2) either node is ON, in state (3) both nodes are OFF. The transition rate matrix and the jump matrix for the chain are provided below.

$$\mathbf{Q} = \begin{pmatrix} -2\beta & 2\beta & 0 \\ \alpha & -(\alpha + \beta) & \beta \\ 0 & 2\alpha & -2\alpha \end{pmatrix} \quad (\text{D.17})$$

$$\mathbf{J} = \begin{pmatrix} 0 & 1 & 0 \\ \frac{\alpha}{\alpha + \beta} & 0 & \frac{\beta}{\alpha + \beta} \\ 0 & 1 & 0 \end{pmatrix} \quad (\text{D.18})$$

The sojourn time in state (1) follows an exponential distribution with rate  $2\beta$  and it corresponds to the length of the ON interval in the joint duty cycle. Instead, the OFF interval of the joint

duty cycle corresponds to the time spent in the class composed of states (2) and (3). This time interval goes from the time at which the chain leaves state (1) until it moves back in. Since the chain moves mandatorily from state (1) to state (2), the time in OFF for the joint duty cycle corresponds to the hitting time from (2) to (1), which can be obtained solving the following system of equations:

$$D_2 = \begin{cases} T_{21} & \text{with probability } p_{21} \\ T_{23} + D_3 & \text{with probability } p_{23} \end{cases} \quad (\text{D.19})$$

$$D_3 = T_{32} + D_2 \quad (\text{D.20})$$

in which we denote with  $D_2$  ( $D_3$ ) the time it takes to move from state (2) (from state (3)) to state (1), with  $T_{ij}$  the time it takes for a direct transition from state  $i$  to state  $j$ , and with  $p_{ij}$  the probability of a jump from state  $i$  to state  $j$  (Equation D.18). From CTMC properties, we know that  $T_{ij}$  are exponential and their rates are given by the corresponding entry of matrix  $\mathbf{Q}$ . By solving Equation D.19 for the first and second moments we get Equations 23 in the main paper. We can also compute the squared coefficient of variation of the time spent in the OFF state of the joint duty cycle, as follows:

$$cv^2 = \frac{2\alpha(6\alpha^2 + 3\alpha\beta + \beta^2)}{(\alpha + \beta)(2\alpha + \beta)^2} + 1 \quad (\text{D.21})$$

## References

- [1] C. Boldrini, M. Conti, and A. Passarella. The stability region of the delay in pareto opportunistic networks. *IEEE Trans. on Mob. Comp.*, 14(1):180–193, 2015.
- [2] A. Chaintreau, P. Hui, J. Crowcroft, C. Diot, R. Gass, and J. Scott. Impact of human mobility on opportunistic forwarding algorithms. *IEEE Trans. on Mob. Comp.*, 6(6):606–620, 2007.
- [3] A. Clauset, C. R. Shalizi, and M. E. Newman. Power-law distributions in empirical data. *SIAM review*, 51(4):661–703, 2009.
- [4] F. M. Dekking. *A Modern Introduction to Probability and Statistics: Understanding why and how*. Springer Science & Business Media, 2005.
- [5] N. Eagle and A. S. Pentland. CRAWDAD dataset mit/reality (v. 2005-07-01). Downloaded from <http://crawdad.org/mit/reality/20050701>, July 2005.
- [6] W. Gao and G. Cao. User-centric data dissemination in disruption tolerant networks. In *IEEE INFOCOM*, pages 3119–3127, 2011.
- [7] A. Passarella and M. Conti. Analysis of individual pair and aggregate intercontact times in heterogeneous opportunistic networks. *IEEE Trans. on Mob. Comp.*, 12(12):2483–2495, 2013.
- [8] J. Scott, R. Gass, J. Crowcroft, P. Hui, C. Diot, and A. Chaintreau. CRAWDAD dataset cambridge/haggle (v. 2009-05-29). Downloaded from <http://crawdad.org/cambridge/haggle/20090529>, May 2009.
- [9] P.-U. Tournoux, J. Leguay, F. Benbadis, J. Whitbeck, V. Conan, and M. D. de Amorim. Density-aware routing in highly dynamic dtns: The rollernet case. *IEEE Trans. on Mob. Comp.*, 10(12):1755–1768, 2011.
